# Supplementary material for: Repairing DoS Vulnerability of Real-World Regexes
Source: arXiv:2010.12450 source file (2022-08-20)
Supplement: Supplementary file 1 [file appendix.tex]

\begin{theorem}
A regular expression that does not contain repetitions runs in constant time.
\end{theorem}
\begin{proof}
We prove that the size of $\mathcal{N}$ is constant.
This proof is by induction on the structure of a regular expression. 
\begin{description}
\item[Base case] $\empty$
	\begin{itemize}
	\item When $r$ is $[C]$, $\mathcal{N} = \{ (p+1, \Gamma) \}$ or a failure. Thus, the size of both $\mathcal{N}$ is one, i.e., constant.
	\end{itemize}	
	\item[Inductive case] $\empty$
	\begin{itemize}
	\item When $r$ is $r_1r_2$, we assume that $(r_1, w, p, \Gamma) \leadsto{} \mathcal{N}$.
	Due to the induction hypothesis, the size of $\mathcal{N}$ is constant.
	Then, $\forall (p', \Gamma') \in \mathcal{N}$, $(r_2, w, p', \Gamma') \leadsto{} \mathcal{N'}$ and the size of $\mathcal{N'}$ is also constant.
	Thus, the size of $\bigcup_{0\leq i< |\mathcal{N}|}\mathcal{N}_i$ is constant.
	\item When $r$ is $r_1 | r_2$, the size of both $\mathcal{N}$ is constant by the induction hypothesis.
	\end{itemize}
	The other cases, i.e., ($r$)$_i$, $\backslash i$, (?:$r$), (?=$r$), (?!$r$), (?<=$r_x$), and (?<!$r_x$) are also proved by the induction hypothesis.
\end{description}
\end{proof}
